# Supplementary material for: Rapformer: Conditional Rap Lyrics Generation with Denoising Autoencoders
Source: arXiv:2004.03965 source file (2020-12-13)
Supplement: Supplementary file 1 [file appendix.tex]

% \section{Additional Model Outputs}\label{sec:examples_appendix}

% In Tables \ref{tab:extra_examples_rap}, \ref{tab:extra_examples_style_transfer_movies} and \ref{tab:extra_examples_style_transfer_news} we display a few additional manually selected model outputs for each of our input domains (rap lyrics, movie summaries and news article summaries) and each of our stripping approaches ({\sc Shuffle} (\model{}), {\sc Drop}, and {\sc Synonym}).

% \section{Demo Song}\label{sec:demo_song}

% We generated lyrics for a demo song by using the abstract of this paper as the input to \model{}. We generated multiple samples, by reshuffling the content words of the abstract multiple times. We sent all sample lyrics to a rap artist, and asked them to record a song using a subset of those lyrics. We allowed for re-arranging and deletion, but no addition of human-created lyrics. The resulting audio file is included in the supplementary material \footnote{Also available at \url{https://bit.ly/37ekn6i}.}, while the final lyrics of the song are in Table \ref{tab:abstract_lyrics}. 

% We also tested the recently released Jukebox algorithm \cite{dhariwal2020jukebox} for end-to-end synthesis of a rap song conditioned on the abstract lyrics. However, our preliminary results were unsatisfactory since it was impossible to tell individual words apart from the generated audio.

% \input{tables/appendix_examples}

% \input{tables/abstract-lyrics}
