# Supplementary material for: Rapformer: Conditional Rap Lyrics Generation with Denoising Autoencoders
Source: arXiv:2004.03965 source file (2020-12-13)
Supplement: Supplementary file 2 [file paper_supplementary_material.tex]

% %
% % File acl2020.tex
% %
% %% Based on the style files for ACL 2020, which were
% %% Based on the style files for ACL 2018, NAACL 2018/19, which were
% %% Based on the style files for ACL-2015, with some improvements
% %%  taken from the NAACL-2016 style
% %% Based on the style files for ACL-2014, which were, in turn,
% %% based on ACL-2013, ACL-2012, ACL-2011, ACL-2010, ACL-IJCNLP-2009,
% %% EACL-2009, IJCNLP-2008...
% %% Based on the style files for EACL 2006 by 
% %%e.agirre@ehu.es or Sergi.Balari@uab.es
% %% and that of ACL 08 by Joakim Nivre and Noah Smith

% \documentclass[11pt,a4paper]{article}
% \usepackage[hyperref]{acl2020}
% \usepackage{times}
% \usepackage{latexsym}
% \usepackage{subfigure}
% \usepackage{graphicx}

% \usepackage{csquotes}

% % \renewenvironment*{displayquote}
% %   {\begingroup\setlength{\leftmargini}{0.3cm}}}
% % % \makeatother


% \usepackage{multirow}
% \usepackage[normalem]{ulem}
% \useunder{\uline}{\ul}{}
% \usepackage{booktabs}

% \usepackage{afterpage}
% \usepackage{boldline}
% \usepackage{cleveref}
% \crefname{section}{§}{§§}
% \Crefname{section}{§}{§§}

% \usepackage[noend,lined,boxed,commentsnumbered]{algorithm2e}

% \renewcommand{\UrlFont}{\ttfamily\small}

% % This is not strictly necessary, and may be commented out,
% % but it will improve the layout of the manuscript,
% % and will typically save some space.
% \usepackage{microtype}

% \usepackage[belowskip=-10pt,aboveskip=2pt]{caption}

% \aclfinalcopy % Uncomment this line for the final submission
% %\def\aclpaperid{***} %  Enter the acl Paper ID here

% %\setlength\titlebox{5cm}
% % You can expand the titlebox if you need extra space
% % to show all the authors. Please do not make the titlebox
% % smaller than 5cm (the original size); we will check this
% % in the camera-ready version and ask you to change it back.

% \newcommand\BibTeX{B\textsc{ib}\TeX}
% \newcommand\model{{\sc Rapformer}}

% % \title{RapFormer: Conditional Rap Lyrics Generation with Denoising Autoencoders}
% % \title{Rapformer: The Rapping Transformer}
% \title{Rapformer: Conditional Rap Lyrics Generation \\ with Denoising Autoencoders \\ \small{Supplementary material}}

% \author{Nikola I. Nikolov$^\dagger$, Eric Malmi$^\ddagger$, Curtis G. Northcutt$^\mathsection$, Loreto Parisi$^\diamond$\\
%   $^\dagger$Institute of Neuroinformatics,
%   University of Zurich and ETH Zurich  \hspace{0.2cm} $^\ddagger$Google  \hspace{0.2cm} $^\mathsection$MIT  \hspace{0.2cm} $^\diamond$Musixmatch \\
%   \texttt{niniko@ini.ethz.ch}\hspace{0.5cm}
%   \texttt{emalmi@google.com} 
%   \hspace{0.5cm} \\ \texttt{cgn@mit.edu}
%   \hspace{0.5cm}
%   \texttt{loreto@musixmatch.com}
%   } 

% \date{}

% \begin{document}
% \maketitle

% \input{appendix}

% \newpage

% \bibliography{bibliography}
% \bibliographystyle{acl_natbib}

% \end{document}
